# Supplementary material for: Extracting the Speed of Sound in Heavy-Ion Collisions: A Study of Quantum-Initiated Fluctuations and Thermalization
Source: arXiv:2501.02777 ancillary file (2025-09-18)
Supplement: Supplementary file 1 [file Supplemental.pdf]

## SUPPLEMENTAL MATERIAL

### 1. *Linear correlation between effective temperature and mean transverse momentum*

The fluid-like fireball created in heavy-ion collisions converts to particles on a hyper-surface $\Sigma$, subject to the freeze-out condition. Through this conversion, the energy and entropy of the expanding fireball are expressed as

$$E = \int_\Sigma d\sigma_\mu T^{\mu 0} = e(T_{\rm eff}) V_{\rm eff}\,, \qquad S = \int_\Sigma d\sigma_\mu s^{\mu} = s(T_{\rm eff}) V_{\rm eff}\,, \tag{6}$$

where $\sigma^\mu$ denotes the normal vector to the freeze-out hyper-surface, and $T^{\mu\nu}$ and $s^\mu$ are the relativistic energy-momentum tensor and entropy flow vector of the fluid, respectively. With respect to the locally equilibrated equation of state (LEOS) that relates energy or entropy density to temperature, the fireball can be effectively reduced to a uniform system characterized by the effective temperature $T_{\rm eff}$ and effective volume $V_{\rm eff}$, as described by the second equation in Eq. (6).

Particles generated from the freeze-out hyper-surface evolve further according to the UrQMD model. The resulting mean transverse momentum $\langle p_T\rangle$ of these final particles is expected to exhibit a linear correlation with the effective temperature $T_{\rm eff}$ on an event-by-event basis. For Pb-Pb collisions, which are approximately 2+1 dimensional due to longitudinal boost invariance, we find that $\langle p_T\rangle^{(i)} \approx 3T_{\rm eff}^{(i)}$, where $i$ labels the event.

In the p-Pb system, however, longitudinal boost invariance no longer holds, introducing ambiguity in the total energy determined by Eq. (6). The effective temperatures obtained using the $(t, x, y, z)$ coordinate system and the $(\tau, x, y, \eta_s)$ Milne coordinate system—where $\tau = \sqrt{t^2 - z^2}$ and $\eta_s = \tanh^{-1}(z/t)$—are found to differ. Despite this discrepancy, solutions from both coordinate systems exhibit a strong linear correlation with $\langle p_T\rangle^{(i)}$ on an event-by-event basis, although the correlation coefficients differ. This difference implies that, in a fireball without boost invariance, the mean transverse momentum of the final-state particles may receive contributions from the kinematic energy associated with longitudinal expansion. As there are two sets of linear relations to the effective temperatures, we consider the realistic energy scale of the fireball that is characterized by the mean transverse momentum in the extraction of the speed of sound lies in between, which gives rise to a range in the linear relation between $\langle p_T\rangle^{(i)}$ and $T_{\rm eff}^{(i)}$. For p-Pb collisions, on an event-by-event basis we find that $\langle p_T\rangle \approx 2.22 \sim 2.8\, T_{\rm eff}$ and $\langle p_T\rangle \approx 2.16 \sim 2.58\, T_{\rm eff}$ for the collision energies $\sqrt{s_{NN}} = 5.02$ TeV and 8.16 TeV, respectively.

### 2. *Derivation of the zero skewness and the zero $\{\delta^5\}_c$ conditions*

According to Eq. (3), $\delta$ can be solved on an event-by-event basis, as

$$\delta = \frac{N_0}{c_s^2 \langle p_T\rangle_0}\Delta_p - \Delta_N, \tag{7}$$

where $c_s^2$ is an unknown parameter to be determined, $\Delta_N = N - N_0$ and $\Delta_p = \langle p_T\rangle - \langle p_T\rangle_0$. With respect to the average over ultra-central collision events, namely,

$$\{\ldots\} = \frac{1}{N_{\rm eve}}\sum_{\rm ieve}^{N_{\rm eve}} \cdots\,, \tag{8}$$

and $N_0$ and $\langle p_T\rangle_0$ the averaged values of $N$ and $\langle p_T\rangle$, one has $\{\delta\} = 0$ by definition. Accordingly, the zero skewness condition is simplified as,

$$\{\delta^3\}_c = \{\delta^3\} - 3\{\delta^2\}\{\delta\} = \{\delta^3\} = 0\,. \tag{9}$$

Substituting Eq. (7) into the condition yields

$$\{\delta^3\} = \left\{ \left(\frac{\Delta_p N_0}{c_s^2\langle p_T\rangle_0} - \Delta_N\right)^3 \right\} \tag{10}$$

$$= (c_s^2)^{-3}\frac{N_0^3}{\langle p_T\rangle_0^3}\{\Delta_p^3\} - 3(c_s^2)^{-2}\frac{N_0^2}{\langle p_T\rangle_0^2}\{\Delta_N\Delta_p^2\} + 3(c_s^2)^{-1}\frac{N_0}{\langle p_T\rangle_0}\{\Delta_N^2\Delta_p\} - \{\Delta_N^3\} = 0\,, \tag{11}$$

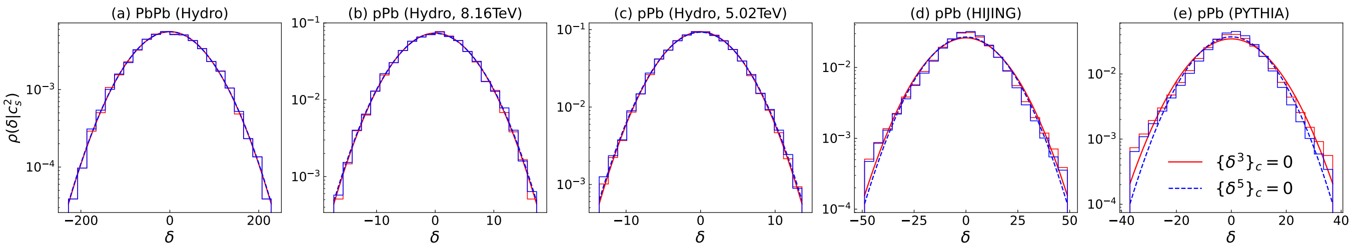


FIG. 4. The normalized probability distribution $\rho(\delta|c_s^2)$ with $c_s^2$ determined by the zero skewness condition $\{\delta^3\}_c = 0$ (red solid histogram). and $\{\delta^5\}_c = 0$ (blue dashed histogram). For comparison, the Gaussian distributions with zero mean and the variance $\{\delta^2\}^{1/2}$ determined with respect to the extracted $c_s^2$ values are shown by lines of the same colors. The quantitative agreement (overlap) between the red and blue curves in the hydrodynamic model results validates the convergence of the analysis in capturing higher-order cumulants associated with Gaussianity.

| $\{\delta^2\}$ | $\{\delta^3\}_c = 0$ | $\{\delta^5\}_c = 0$ |
|---|---|---|
| PbPb (Hydro, 5.02TeV) | $5076 \pm 140$ | $5108 \pm 145$ |
| pPb (Hydro, 8.16 TeV) | $29.2 \pm 0.4$ | $29.7 \pm 0.4$ |
| pPb (Hydro, 5.02 TeV) | $18.1 \pm 0.2$ | $18.5 \pm 0.2$ |
| pPb (PYTHIA, 5.02 TeV) | $233.3 \pm 1.8$ | $220.2 \pm 1.8$ |
| pPb (HIJING, 5.02 TeV) | $133.2 \pm 0.3$ | $115.5 \pm 0.2$ |

TABLE II. A summary of the second order moment $\{\delta^2\}$ of the $\delta$-distribution from different collision systems, with respect to the speed of sound solved from the condition of zero skewness and $\{\delta^5\}_c = 0$.

which leads to Eq. (4):

$$(c_s^2)^3 \frac{\{\Delta_N^3\}}{N_0^3} - 3(c_s^2)^2 \frac{\{\Delta_N^2 \Delta_p\}}{N_0^2 \langle p_T \rangle_0} + 3c_s^2 \frac{\{\Delta_N \Delta_p^2\}}{N_0 \langle p_T \rangle_0^2} - \frac{\{\Delta_p^3\}}{\langle p_T \rangle_0^3} = 0. \tag{12}$$

In addition to the zero skewness condition, if one further considers the Gaussianity of $\delta$ to be satisfied in higher order cumulants, such as the fifth order cumulant $\{\delta^5\}_c$, in the same manner inserting Eq. (7) into the condition $\{\delta^5\}_c = 0$, one gets

$$(c_s^2)^5 \frac{\{\Delta_N^5\}}{N_0^5} - 5(c_s^2)^4 \frac{\{\Delta_N^4 \Delta_p\}}{N_0^4 \langle p_T \rangle_0} + 10(c_s^2)^3 \frac{\{\Delta_N^3 \Delta_p^2\}}{N_0^3 \langle p_T \rangle_0^2} - 10(c_s^2)^2 \frac{\{\Delta_N^2 \Delta_p^3\}}{N_0^2 \langle p_T \rangle_0^3} + 5c_s^2 \frac{\{\Delta_N \Delta_p^4\}}{N_0 \langle p_T \rangle_0^4} - \frac{\{\Delta_p^5\}}{\langle p_T \rangle_0^5} = 0. \tag{13}$$

In all the collision systems we have considered, the distributions of $\mathcal{P}(\delta|c_s^2)$ with the value of speed of sound solved according to Eq. (13) are shown in Fig. 4 as blue histograms, and the corresponding Gaussian distributions are shown as blue dashed lines. Comparing to the same results obtained from $\{\delta^3\}_c = 0$ (red color in Fig. 4), we observe a trend of convergence in the hybrid hydrodynamic models, e.g., the second order moments of the $\delta$-distrbutions from the two conditions are compatible within statistical uncertainties (Table. II).
